# Supplementary material for: Frugal Byzantine Computing
Source: arXiv:2108.01330 source file (2021-08-03)
Supplement: Supplementary file 1 [file SI_RB.tex]

% \renewcommand{\figurename}{Algorithm}
% \begin{figure}[p]
%     \caption{Fast Reliable Broadcast}
\begin{lstlisting}[columns=fullflexible,breaklines=true,float=p,caption={Fast Reliable Broadcast},label={alg:b_fast-rb}]
Shared:
Value, L1Proof, L2Proof - @$n \times n$@ array of "slots"; each slot is a 2-tuple (msg, sgn) of SWMR atomic registers, initialized to @$(\bot,\bot)$@.  
    
Sender code:
broadcast(m) {
    Value[me,me].msg.write(m) @\label{line:bdcast_m}@
}

Replicator code:
state = WaitForSender //@$\in$@{WaitForSender,WaitForL1Proof,WaitForL2Proof}
//let q be the broadcaster

if (state == WaitForSender) {
    m = Value[q,q].msg.read() @\label{line:read_m}@
    if (m @$\neq$@ @$\bot$@) {
        Value[me,q].msg.write(m)
        In the background {
            @$\sigma$@ = compute signature for m @\label{line:sign_m}@
            Value[me,q].sgn.write(@$\sigma$@) 
        }
        state = WaitForL1Proof @\label{line:changeStateL1}@
}   }

if (state == WaitForL1Proof) {
    checkedVals = @$\emptyset$@
    for t @$\in \Pi$@ {
        other = Value[t,q].(msg,sgn).read();
        if (other.msg == m and other.sgn is a valid signature for m)
            checkedVals.add((t,other))
    }


    if (size(checkedVals) @$\geq n-f$@ ) {@\label{line:b_checkL1proof}@
        L1Proof[me,q].msg.write(checkedVals)@\label{line:b_writel1prf}@
        L1others = L1Proof[t,q].(msg,sign).read() for t in @$\Pi$@ // Read all L1 Proofs@\label{line:readlallL1}@
        if (@$\not\exists$@ t s.t. (L1others[t] is a valid L1 proof and L1others[t] is not for m)) {// no L1 proof contradicts mine@\label{line:checkbeforesignl1}@
            @$\sigma$@ = compute signature for checkedVals
            L1Proof[me,q].sgn.write(@$\sigma$@)@\label{line:sign_l1}@
            state = WaitForL2Proof
}   }   }
    
if (state == WaitForL2Proof) {
    checkedL1Prfs = @$\emptyset$@ @\label{line:start_l1check}@
    for t in @$\Pi$@ {
        prf = L1Proof[t,q].(msg,sgn).read();@\label{line:b_readL1prf}@
        if (prf.sgn is a valid signature for prf.msg and prf.msg is a valid L1 proof for m)
            checkedL1Prfs.add((t,prf)) @\label{line:end_l1check}@
    
    if (size(checkedL1Prfs) @$\geq n-f$@) {
        L2Proof[me,q].msg.write(checkedL1Prfs)@\label{line:b_writeL2proof1}@}
}   }

In the background {/another task/...
    L2others =  L2Proof[t,q].msg.read() for t in @$\Pi$@ 
    if ((@$\exists$@ t s.t. L2others[t].msg is a valid L2 proof) and (L2Proof[me.q].msg @$== \bot$@)) { @\label{line:check-otherL2}@
        L2Proof[me,q].msg.write(L2others[t].msg)@\label{line:writeL2fromother}@
}


Receiver code:
try_deliver(q) {
    others = Value[t,q].msg.read() for t in @$\Pi$@
    proofs = L2Proof[t,q].msg.read() for t in @$\Pi$@
    if (others[t].msg has the same value, msg, for all t in @$\Pi$@) { // Fast Path @\label{line:b_fast-check}@
        return msg @\label{line:b_fast-return}@
    } else if (proofs contains at least @$n-f$@ valid L2 proofs for the same value, msg) { @\label{line:b_slow-check}@ // Slow Path 
        return msg @\label{line:b_slow-return}@
    } else {
        return @$\bot$@
}   }                
\end{lstlisting}
    % 
% \end{figure}

To broadcast a message $m$, the sender $q$ writes $m$ in its message sub-slot. In contrast to \neb, the broadcaster is no longer required to compute and write a signature for $m$.
This is because once a correct receiver delivers a message, an algorithm needs to allow future correct receives to deliver the same message (totality + consistency), regardless of the behaviour of the broadcaster. 
E.g., consider the case in which a correct receiver $r$ delivers $m$ via the fast-path from a Byzantine broadcaster. Let this broadcaster no longer append a signature. An implementation must allow a correct receiver $r'$ to also deliver $m$, tolerating up to $f$ Byzantine replicators who might change their values and without relying on the signature of the broadcaster. 
% A concrete scenario: sender $q$ is faulty, it broadcasts $m$ yet it does not append a signature for $m$. A correct receiver, $r_1$, delivers message $m$ via the fast-path. Up to $f$ Byzantine replicators remove $m$ from their slot so that no correct receiver, say $r_2$, can deliver a message via the fast-path. Totality requires $r_2$ to eventually deliver $m'$, while consistency require $m'$ to be the same as the message $r_1$ delivered, $m'=m$.

Upon reading a message $m$ from the broadcaster's slot, a correct replicator, $r$ copies this value in its slot, computes and writes its signature for message $m$.

Process $r$ constructs an L1 proof with at least $n-f$ signed values for $m$ and writes it in its L1Proof slot. It then reads all L1Proof slots, if there is no L1 proof consisting of at least $n-f$ signed values for $m' \neq m$, it computes and appends its signature for its own L1 proof.
This step ensures no two correct replicators construct a signed, valid L1 proof for different values. %; which would then allow conflicting L2 proofs.

When process $r$ reads $n-f$ signed, valid L1 proofs for $m$, it constructs its L2 proof with these values.
Process $r$ is also able to copy a valid L2 proof from another replicator in its own slot given it has not previously written its L2 proof. 

No two correct replicators append their signature to their L1 proof once they read a valid L1 proof, i.e., a set of $n-f$ signed values, for a different value than its own. This means that $n-f$ correct replicators build a signed L1 proof for at most one value. Hence, a valid L2 proof can only exist for one value since it requires $n-f$ signed, valid L1 proofs (and there are at most $f$ Byzantine replicator processes and signatures are unforgeable).

A receiver $p$ reads the Value and L2Proof slots of the replicators.
There are two ways in which $p$ can deliver: (1) (the fast path) if there is unanimity, all $n$ replicators copied the same message $m$; (2) (the slow path) if there exist $n-f$ valid L2 proofs for the same message $m$.

To ensure totality holds we require the delivery via slow path to happen only once $n-f$ L2 proofs are present. This is such that at least one correct replicator wrote one of the existing L2 proofs. This proof is ensured to be preserved in its L2 slot regardless of the behaviour of the $f$ Byzantine replicators, so that the remaining $n-f-1$ correct replicators can copy the L2 proof over.

\begin{lemma}[Validity]
If a correct process $p$ broadcasts $m$, then \trydel($p$) will eventually return $m$ at any correct process $q$. 
\end{lemma}

\begin{proof}
%  Assume by contradiction that there exists some correct receiver who does not deliver $m$.
% It is either the case that the receiver does not read unanimity of slots for $m$ or it does not read at least $n-f$ valid L2 proofs.

Let $p$ be a correct sender that broadcasts $m$ and consider a correct receiver $q$ that tries to deliver $p$'s message.  

Since $p$ is correct, upon broadcasting $m$, it writes $m$ in its slot, Value[p,p] (line~\ref{line:bdcast_m}). By Observation~\ref{obs:no-overwrite}, $m$ will remain in that slot forever. 
Therefore, all replicators eventually read $m$ (line~\ref{line:read_m}) and no other message from $p$.

If all replicators are correct and they copy $m$ in a timely manner, then $q$ is able to return $m$ via the if-branch of the conditional statement (line~\ref{line:b_fast-check}). 

Otherwise, we consider at most $f$ Byzantine replicator processes.
Since $p$ is correct and broadcasts one value, $m$, no correct replicator process writes any other value $m'\neq m$ into its Values[*,p].msg slot. The $n-f$ correct replicator compute their signature for $m$, write it into their own Value[*,p].sgn and change their state to WaitForL1Proof (lines~\ref{line:sign_m}--~\ref{line:changeStateL1}). 

Eventually, each correct process will collect at least $n-f$ copies of $m$ in its checkedVals set, and write these into its L1Proof[*,p].msg slot (line~\ref{line:b_writel1prf}).
Every correct process reads the L1Proof[*,p].msg slots of the other processes to make sure no other valid L1 proof exists for a different value $m'\neq m$. If that is the case, each correct process appends its signature to the previously written message, L1Proof[*,p].sgn (line~\ref{line:sign_l1}) and change its state to WaitForL2Proof.
This is ensured to happen since all correct replicators support $m$, there are at most $f$ Byzantine processes, and signatures are unforgeable. That is, the Byzantine replicators cannot form a valid L1 proof for $m'\neq m$, i.e., a set of $n-f$ signed values for $m' \neq m$. 

All correct processes will eventually read at least $n-f$ valid L1 proofs for $m$ and add these to the checkedL1Prfs set (lines~\ref{line:start_l1check}--~\ref{line:end_l1check}). Every correct process either writes this set into its L2 proof slot, L2Proof[*,q].msg (line~\ref{line:b_writeL2proof1}) or copies a valid L2 proof it reads from another replicator in its L2 proof slot (line~\ref{line:writeL2fromother}).

This enables a receiver to return $m$ via the else-if-branch of the conditional statement (line~\ref{line:b_slow-check}). 

% This contradicts our assumption that a correct receiver does not deliver $m$ from $p$.
\end{proof}

\begin{lemma}[Consistency]
If $p$ and $q$ are correct processes (potentially the same process), $p$ delivers $m$ from $r$ and $q$ delivers $m'$ from $r$, then $m{=}m'$. 
\end{lemma}

\begin{proof}
Assume by contradiction that consistency does not hold; assume correct process $p_1$ delivers $m_1$ from $q$, while correct process $p_2$ delivers $m_2 \ne m_1$ from $q$. 
	
Since $p_1$ and $p_2$ are correct, they must have read either at least $n-f$ valid L2 proofs or unanimity of values before delivering $m_1$ and $m_2$ respectively.

Assume first \textit{wlog} that $p_1$ delivers $m_1$ using the if-branch of the conditional statement (line~\ref{line:b_fast-check}). Then $p_1$ must have seen $m_1$ in $n$ replicator slots.
Assume now that $p_2$ delivers $m_2$ using the same check; then, $p_2$ must have seen $m_2$ in $n$ replicator slots. This means that all $n$ replicators must have changed their written value, either from $m_1$ to $m_2$, or vice-versa; this is impossible since at least $n-f$ of the replicators are correct and never change their written value (Observation~\ref{obs:no-overwrite}).

Process $p_2$ must have then delivered $m_2$ using the else-if check instead (line~\ref{line:b_slow-check}); then, $p_2$ must have seen at least $n-f$ valid L2 proofs for $m_2$ in the replicator slots. 
In order to construct a valid L2 proof for $m_2$, one requires a signed set of $n-f$ L1 proofs for $m_2$. This means that at least one correct replicator must have constructed an L1 proof for $m_2$. Since correct replicators only construct L1 proofs for their own value, it must be that this replicator changed its value from $m_1$ to $m_2$ (or from $m_2$ to $m_1$) which is impossible by Observation~\ref{obs:no-overwrite}.
% Since all correct replicators, $n-f$, have written values for value $m_1$, these processes will only construct an L1 proof for value $m_1$. Consequently, Byzantine processes cannot build a valid L2 proof for $m_2$ as it requires at least $n-f$ valid L1 proofs for $m_2$. 

So it must be that $p_1$ and $p_2$ deliver $m_1$ and $m_2$, respectively, using the else-if-branch of the conditional statement. In this case $p_1$ sees $n-f$ valid L2 proofs for $m_1$, while $p_2$ seems $n-f$ valid L2 proofs for $m_2$.
Let $\mathcal{P}$ and $\mathcal{P'}$ be any of those valid proofs for $m_1$ and $m_2$ respectively. $\mathcal{P}$ (resp. $\mathcal{P'}$) consists of at least $n-f$ valid L1 proofs. A valid L1 proof holds the signature of the replicator who wrote it. Therefore, at least one of those proofs was created by some correct process $r_1$ (resp. $r_2$). Since $r_1$ (resp. $r_2$) is correct, it must have written the L1 proof for $m_1$ (resp. for $m_2$) to its L1Proof.msg slot (line~\ref{line:b_writel1prf}). Note that after writing to their slot, in the WaitForL1Proof state, correct processes read \emph{all} L1 proof slots (line~\ref{line:readlallL1}). Thus, both $r_1$ and $r_2$ read all L1 proof slots before signing their L1 proof for $m_1$ (resp. $m_2$). 

Assume without loss of generality that $r_1$ wrote its L1 proof for $m_1$ before $r_2$ wrote its L1 proof for $m_2$; by Observation~\ref{obs:no-overwrite}, it must then be the case that $r_2$ later saw both the L1 proof for $m_1$ and the L1 proof for $m_2$ when it read all L1Proof slots (line~\ref{line:readlallL1}). Since $r_2$ is correct, it cannot have then signed its L1 proof for $m_2$ (the check at line~\ref{line:checkbeforesignl1} failed). 
Since there are not two valid L2 proofs for different values, $m_1$ and $m_2$, there can't be $n-f$ copies of valid proofs for different values.
We have reached a contradiction: $p_1$ does not deliver $m_1$ or $p_2$ does not deliver $m_2$.

\end{proof}

\begin{lemma}[Integrity] 
If a correct process delivers $m$ from $p$ and $p$ is correct, then $p$ must have broadcast $m$.
\end{lemma}

\begin{proof}
A correct receiver deliver a non-empty value either when (a) it sees the same value in all replicator Value.msg slots or (b) it sees at least $n-f$ valid L2 proofs in L2Proof.msg slots.

Case (a) occurs when all replicators (including $n-f$ correct replicators) have written $m$ in their Value slot. Given correct processes only write the value they read in slot of the broadcaster $p$ and given $p$ is correct, it only writes a value in Value[p,p] upon a broadcast event. Then, $p$ must have broadcast $m$.

Case (b) occurs when the receiver sees $n-f$ valid L2 proofs for $m$. Let any of these valid L2 proofs the receiver sees for $m$ be denoted $\mathcal{P}$. $\mathcal{P}$ consists of at least $n-f$ L1 proofs for $m$. Each L1 proof consists of at least $n-f$ signed copies of $m$. This means, there is at least one correct replicator that contributes with a signed value $m$. Such a correct process only copies a value it reads from the broadcaster's slot, Value[p,p].msg. Since we assume the broadcaster $p$ is correct, $p$ only writes a value in its slot upon a broadcast event. Then, $p$ must have broadcast $m$.

\end{proof}

\begin{lemma}[Totality] 
If some message $m$ is delivered by any correct process, every correct process eventually delivers a message.
%alt: if a corr dels m all corr evtly del m' for some m'
\end{lemma}

\begin{proof}
Let $p_1$ be a correct process such that $p_1$ delivers $m_1$ from $q$. We show that all correct process must eventually deliver $m_2$ from $q$, for some $m_2$.

Assume by contradiction that there exists some correct process $p_2$ who does not deliver $m_2$ from $q$, for any $m_2$. 

Since $p_1$ delivers $m_1$ from $q$, then $p_1$ must have either (a) seen $m_1$ in all Values slots of the replicators or (b) seen at least $n-f$ valid L2 proofs for $m_1$.
\dalia{here should make proof for: l2 proof can only be for 1 value?}%. $\mathcal{P_1}$ 

Case (a). When $p_1$ delivers $m_1$ via the if-statement, it must be the case that $n$ replicators have the same value written, and in particular $n-f$ correct replicator processes have the same value written, $m_1$. The correct replicators, will eventually construct an L1 proof with each others' Value[*,q]. Since there are at most $f$ Byzantine replicators, Byzantine processes cannot forge signatures, and correct replicators do not change their written value, they have insufficient data to construct a valid L1 proof for $m_2 \neq m_1$. The correct processes append a signature for their L1 proof since no conflicting L1 proof can exist.
Any correct replicator is then able to construct an L2 proof for $m_1$ or copy an L2 proof for $m_1$ from another correct replicator that constructs it first.
Process $p_2$ is then able to read $n-f$ valid L2 proofs for $m_1$ and hence deliver $m_1$ via the else-if statement.

Case (b). Since $p_1$ sees at least $n-f$ valid L2 proofs for $m_1$, it must be the case that at least one of these proofs is written by a correct replicator, say $r$. By Observation~\ref{obs:no-overwrite}, this L2 proof stays in $r$'s slot forever. 
Since there are $n-f$ correct replicators in the system, these processes either try to construct their own L2 proof (which can only be for $m_1$\dalia{does this need backup?}), or copy an existing valid L2 proof from another replicator (line~\ref{line:writeL2fromother}). All correct replicators are at least able to eventually read $r$'s valid L2 proof and copy it over.
% even in the case when $n-f-1$ processes are Byzantine and remove their L2 proofs.

Consequently, a valid L2 proof for $m_1$ exists in $n-f$ replicator slots and $p_2$ is able to deliver $m_1$ via the else-if statement. 

% *******************
% \dalia{to think about this case - what if byz construct a valid l2 proof and remove it; can one be sure to ever be able to construct another??} 

% Take 5 replicators p0,...,p4
% consider byz primary broadcast m
% correct replicator p2 copies m
% now byz changes to m'
% correct replicators p3,p4 copy m'
% p0,p1 Byz initially have m
% all add their signatures
% p2 constructs an L1 set from p0,p1,p2 for m
% there is no conflicting L1; it adds its signature
% other 2 correct p3,p4 cannot form any L1 proof
% say byzantine form an L1 proof p0,p1,p2 for m
% yet they do not let p2 sufficient time so that it reads and writes an l2 proof
% yet any of the Byzantine processes can construct an L2 proof

% now a correct receiver delivers
% and the proof is removed

% no other correct receiver can deliver 

% (i think this was solved in previous RB by writing an L2 once can read it; before delivery;
% yet now receivers are disconnected from each other!)

% updated alg with Naama's suggestion; added the background task at replicators and adjusted the else-if conditions at receiver
\end{proof}
