# Supplementary material for: Frugal Byzantine Computing
Source: arXiv:2108.01330 source file (2021-08-03)
Supplement: Supplementary file 2 [file SI_RB_from_CB.tex]

\begin{lstlisting}[columns=fullflexible,breaklines=true,keywords={if,when,return,else,for},float=ht,caption={Reliable Broadcast Algorithm},label={alg:fast-rb-from-cb}]
Shared:
Init - instance of BCB with sender s (same as RB)
Echo - array of n BCB instances; Echo[i] is BCB with sender i
Ready - array of n SWMR registers; Ready[i] has writer i

Sender code:
broadcast(m) {
    Init.broadcast(m)   }

Replicator code:
state = WaitForSender //@$\in$@{WaitForSender,WaitForEchos}

if (state == WaitForSender) {
    if (delivered m from Init) { // should also say here: "and not send ECHO yet"?
        Echo[me].broadcast(m)
        state = WaitForEchos }  }
     
if (state == WaitForEchos) {
    when (deliver m from Echo[i] and m has a valid signature by i) {
        add (i,m) to EchoSet    }
    
    if (@$\exists m$:@ EchoSet contains @$n-f$@ elements (*,m)) {
        ReadySet = set of @$n-f$@ signed echo messages @for@ m
        ready = true
        Ready[me].write(ReadySet)   }   }   

In the background {
    if (!ready) {
        others = Ready[i].read() for i in @$\Pi$@ // Read all Values
        if (@$\exists i:$@ others[i] is a valid ReadySet) {
            ready = true
            Ready[me].write(others[i])  }   }   }

Receiver code:
try_deliver(s) {
    others = Ready[i].read() for i in @$\Pi$@ 
    if (delivered @$n$@ matching values m from Echo[i] and !delivered) {
        delivered = true
        return m   }
    if (others contains @$n-f$@ valid ReadySet @for@ the same value m and !delivered) {
        delivered = true
        return m    }
    return @$\bot$@ }                
\end{lstlisting}
    % 
% \end{figure}

The processes communicate by sharing an array \textit{Ready}: \textit{Ready[t]} is an atomic SWMR register where process $t$ can write to, and by using instances of \neb{} (BCB). A sender broadcasts using an Init BCB instance, while each replicator broadcasts using an Echo BCB instance.

To broadcast a message, the sender $s$ Init broadcasts $m$. Upon delivering a sender's message, $m$, every replicator Echo broadcasts $m$.
Each replicator delivers a signed message $m$ from another replicator's Echo. Upon delivering $n-f$ such messages, a replicator constructs a \textit{ReadySet} with these values and writes it in its \textit{Ready} register.
In the background, replicators read the \textit{Ready} registers of other replicators and copy into their \textit{Ready} register any valid \textit{ReadySet} they read.

A receiver $p$ reads the \textit{Ready} registers of the replicators and delivers messages from Echo of the replicators. There are two ways in which process $p$ can deliver the sender's message $m$: (1) [fast path] if process $p$ delivers message $m$ from Echo of all $n$ replicators or (2) [slow path] if $n-f$ replicators wrote a valid \textit{ReadySet} for $m$.
A signature-less fast path occurs when the delivery of the Echo messages by $p$ is done via the fast path of \neb, and the delivery of the Init message by the replicators is done via the fast path of \neb. This is the case when replicators are timely with replicating messages and when the replicators are not faulty.

To ensure totality holds we require a correct receiver $p$ to deliver $m$ via slow path only once it reads $n-f$ \textit{ReadySets}. This is such that at least one correct replicator, say $r$, wrote one of these sets. Replicator $r$'s \textit{ReadySet} is ensured to be preserved in its slot regardless of the behaviour of the $f$ Byzantine replicators. The remaining $n-f-1$ correct replicators are able to copy this set over and allow future receivers to deliver a message as well.

\begin{invariant}\label{invariant:rbValidSets}
    Let $S$ and $S'$ be two valid ReadySets for $m$ and $m'$, respectively. Then, $m=m'$.
\end{invariant}
\begin{proof}
    By contradiction. Assume there exist valid ReadySets $S$ and $S'$ for different values $m\ne m'$.
    Set $S$ (resp. $S'$) consists of at least $n-f$ signed $m$ (resp. $m'$) messages. 
    Then there exist correct replicators $r$ and $r'$ such that $r$ Echo broadcasts $m$ and $r'$ Echo broadcasts $m'$. This is impossible since correct replicators only invoke Echo.broadcast(*) once they have delivered some message from the Init \neb{} (BCB) instance. By the consistency property of \neb, $m$ must be equal to $m'$.
\end{proof}

\begin{lemma}[Validity]
If a correct process $s$ broadcasts $m$, then \trydel($s$) will eventually return $m$ at any correct process $p$. 
\end{lemma}

\begin{proof}
Assume the sender $s$ is correct and broadcasts $m$.
This implies the sender broadcasts $m$ through its Init BCB instance.
By the validity property of \neb, all correct replicators will eventually deliver $m$ from Init. Then, all correct replicators will broadcast $m$ through their Echo BCB instances. By the validity* property of \neb, all correct replicators will thus eventually deliver signed messages for $m$ from each other's Echo; thus every correct replicator will be able to either (a) create a valid ReadySet and write it into its Ready register or (b) copy a valid ReadySet into its Ready register. Thus, correct receivers will eventually be able to read at least $n-f$ valid ReadySets for $m$ and deliver $m$ via the slow path.    
\end{proof}

\begin{lemma}[Consistency]
If $p$ and $p'$ are correct processes (potentially the same process), $p$ delivers $m$ from $s$ and $p'$ delivers $m'$ from $s$, then $m{=}m'$. 
\end{lemma}
\begin{proof}
    By contradiction. Let $p,p'$ be two correct receivers. Let $p$ deliver $m$ and $p'$ deliver $m' \neq m$ from $s$. We consider 3 cases: (1) $p$ and $p'$ deliver their messages via the fast path, (2) $p$ and $p'$ deliver their messages via the slow path, and (3) (wlog) $p$ delivers via the fast path and $p'$ delivers via the slow path.
    
    (1) $p$ and $p'$ must have delivered $m$ and $m'$ respectively, from Echo of $n$ replicators. Thus, there exists at least one replicator $r$ such that $p$ delivered $m$ from $r$'s Echo and $p'$ delivered $m'$ from $r$'s Echo. This is impossible by the consistency property of \neb.
    
    (2) $p$ and $p'$ must have each read $n-f$ valid ReadySets for $m$ and $m'$, respectively. This is impossible by Invariant~\ref{invariant:rbValidSets}.
    
    (3) $p'$ read at least one valid ReadySet for $m'$. Thus, at least one correct replicator $r$ must have Echo broadcast $m'$. Process $p$ delivered $m$ from Echo of all $n$ replicators, which includes $r$. This is impossible by the consistency property of \neb.
\end{proof}

\begin{lemma}[Integrity] 
If a correct process delivers $m$ from $s$ and $s$ is correct, then $s$ must have broadcast $m$.
\end{lemma}
\begin{proof}
    Let $p$ be a correct receiver that delivers $m$ from a correct sender, $s$. We consider 2 cases (1) $p$ delivers $m$ via the fast path and (2) $p$ delivers $m$ via the slow path.
    
    (1) Fast Path. $p$ must have delivered $m$ from Echo of at least one correct replicator $r$. Replicator $r$ Echo broadcasts $m$ upon delivery of $m$ from Init. By the integrity property of \neb, $s$ must have Init broadcast $m$.
    A correct sender only invokes Init broadcast $m$ upon a broadcast event for $m$.
    
    (2) Slow Path. $p$ must have read at least one valid ReadySet for $m$. Thus, at least one correct replicator $r$ must have Echo broadcast $m$. Same argument as above.
\end{proof}

\begin{lemma}[Totality] 
If some message $m$ is delivered by any correct process, every correct process eventually delivers a message.
\end{lemma}    
\begin{proof}
    Let $p$ be a correct receiver that delivers $m$ from a sender $s$. We consider 2 cases (1) $p$ delivers $m$ via the fast path and (2) $p$ delivers $m$ via the slow path.
    
    (1) Fast Path. $p$ must have delivered $m$ from Echo of all $n$ replicators, which include $n-f$ correct replicators. These $n-f$ correct replicators must also receive each other's Echo messages (by the validity property of \neb). Therefore, each of them will be able to construct and write a valid ReadySet to its Ready register (or copy a valid set into its Ready register). Thus, every correct receiver will eventually read $n-f$ valid ReadySets for $m$ and deliver $m$ via the slow path.
    
    (2) Slow Path. $p$ must have read valid ReadySets for $m$ from $n-f$ replicators, which must include at least one correct replicator $r$. Since $r$ is correct, $r$ will never remove its ReadySet for $m$. Thus, every correct replicator will eventually either (a) copy $r$'s ReadySet to their own Ready slots or (b) construct and write a ReadySet to their Ready slots. Note that by Invariant~\ref{invariant:rbValidSets}, all valid ReadySets must be for the same value $m$. Thus, every correct receiver will eventually read $n-f$ valid ReadySets for $m$ and deliver $m$ via the slow path.
\end{proof}
