# Supplementary material for: Frugal Byzantine Computing
Source: arXiv:2108.01330 source file (2021-08-03)
Supplement: Supplementary file 3 [file SI_RBsign.tex]

% \renewcommand{\figurename}{Algorithm}
% \begin{figure}[p]
%     \caption{Fast Reliable Broadcast}
\begin{lstlisting}[columns=fullflexible,breaklines=true,float=ht,caption={Reliable Broadcast with Sender Signature},label={alg:s_fast-rb}]
Shared:
Value, L1Proof - @$n \times n$@ array of "slots"; each slot is a 2-tuple (msg, sgn) of SWMR atomic registers, initialized to @$(\bot,\bot)$@.  
    
Sender code:
broadcast(m) {
    @$\sigma$@ = compute signature for m
    Value[me,me].(msg,sgn).write(m,@$\sigma$@) @\label{line:s_bdcast_m}@
}

Replicator code:
state = WaitForSender //@$\in$@{WaitForSender,WaitForL1Proof}
//let q be the broadcaster

if (state == WaitForSender) {
    val = Value[q,q].(msg,sgn).read() @\label{line:s_read_m}@
    if (val.msg @$\neq$@ @$\bot$@ and val.sgn is a valid signature for val.msg) {
        Value[me,q].msg.write(val)
        others = Value[t,q].msg.read() for t in @$\Pi$@ // Read all Values
        if (@$\not\exists$@ t s.t. (others[t].msg @$\neq$@ val.msg and others[t].sgn is a valid signature for others[t].msg )) {// no validly signed value by broadcaster contradicts mine@\label{line:s_checkbeforesign}@
            @$\sigma$@ = compute signature for val
            Value[me,q].sgn.write(@$\sigma$@)@\label{line:s_sign_val}@
            state = WaitForL1Proof
}   }   }       
        
if (state == WaitForL1Proof) {
    checkedVals = @$\emptyset$@
    for t @$\in \Pi$@ {
        other = Value[t,q].(msg,sgn).read();
        if (other.msg == val and other.sgn is a valid signature for others.msg)
            checkedVals.add((t,other))
    }


    if (size(checkedVals) @$\geq n-f$@ )@\label{line:s_b_checkL1proof}@
        L1Proof[me,q].msg.write(checkedVals)@\label{line:s_b_writel1prf}@
}   

In the background {/another task/...
    L1others =  L1Proof[t,q].msg.read() for t in @$\Pi$@ 
    if ((@$\exists$@ t s.t. L1others[t].msg is a valid L1 proof) and (L1Proof[me.q].msg @$== \bot$@)) @\label{line:s_check-otherL1}@
        L1Proof[me,q].msg.write(L1others[t].msg)@\label{line:s_writeL1fromother}@
}


Receiver code:
try_deliver(q) {
    proofs = L1Proof[t,q].msg.read() for t in @$\Pi$@
     if (proofs contains at least @$n-f$@ valid L1 proofs for the same value, msg) { @\label{line:s_b_slow-check}@ // Slow Path 
        return msg @\label{line:s_b_slow-return}@
    } else {
        return @$\bot$@
}   }                
\end{lstlisting}
    % 
% \end{figure}

Here we assume the sender appends a signature and then we have total of n replicator signatures (and not 2n).
It would be nice to prove that the presence of a fast path adds extra costs -- one can deliver without seeing whether broadcaster appends a value; unless the replicators replicate a value only upon a valid signature check but this is not sufficient; can be the case that fp goes through; yet Byzantine replicator has a validly signed m' appended after fp delivery st no L1 can be constructed)

Once the replicator copies a validly signed value from the broadcaster, a replicator only appends its signature if there is no contradicting value it reads from the other replicators.

The set of $n-f$ correct replicators are ensured to add a signature to at most one value copied from the broadcaster.

If write of a correct process $p_1$, $W_1$, happens before the write of correct process $p_2$, $W_2$, process $p_2$ is ensured to read both $p_1$ and $p_2$'s value. 
When the writes are concurrent, they cannot miss each other. At least one must read the other's value.

Proof sketch
Process $p_1$, performs the following actions $W_1$ and $R_2$.
Process $p_2$ performs the following actions $W_2$ and $R_1$.
\begin{itemize}
    \item $W_1$ < $R_2$ (process $p_1$ first writes, then performs read all)
    \item $W_2$ < $R_1$ (process $p_2$ first writes, then performs read all)
    \item $R_2$ < $W_2$ (for $p_1$ to miss $p_2$'s write, it must have read before the write)
    \item $R_1$ < $W_1$ (for $p_2$ to miss $p_1$'s write, it must have read it before the write)
\end{itemize}
Now we get $W_1 < R_2 < W_2 < R_1 < W_1$, no linearization point.

Hence there will be at most a valid $L1$ proof for a single message.

For totality to hold, we use the same trick, one waits for $n-f$ valid $L1$ proofs to deliver a message; when a (correct) replicators reads a valid $L1$ message, this replicator copies it over.
