# Supplementary material for: Frugal Byzantine Computing
Source: arXiv:2108.01330 source file (2021-08-03)
Supplement: Supplementary file 4 [file appendix-relatedwork.tex]

\section{APPENDIX: Additional Related Work}\label{app:related-work}
